# Supplementary material for: The Ophiuchus DIsc Survey Employing ALMA (ODISEA). Substructures as a function of SED Class and disc mass in 100 systems
Source: arXiv:2604.19246 source file (2026-09-03)
Supplement: Supplementary file 1 [file supplementary.tex]

\documentclass{aa}

\usepackage{graphicx}
\usepackage{comment}
%%%%%%%%%%%%%%%%%%%%%%%%%%%%%%%%%%%%%%%%
\usepackage{txfonts}
\usepackage{caption}
\usepackage{subcaption}
\usepackage{xcolor}

\usepackage{graphicx}
%%%%%%%%%%%%%%%%%%%%%%%%%%%%%%%%%%%%%%%%
\usepackage{lipsum} 
\usepackage{gensymb}
\usepackage{txfonts}
\usepackage{amssymb}
\usepackage{amsmath}
\usepackage{booktabs}
\usepackage{dcolumn}
\usepackage{sidecap}
\usepackage{subfig}
\usepackage{multirow}
\usepackage{threeparttablex}
\usepackage{longtable}
\usepackage{xcolor}
\usepackage{natbib}
\usepackage{pdflscape}
\usepackage{upgreek}
\usepackage{lscape}
\bibpunct{(}{)}{;}{a}{}{,}
\usepackage{array}
\newcolumntype{H}{>{\setbox0=\hbox\bgroup}c<{\egroup}@{}}

% \bibliographystyle{aa}
%%%%%%%%%%%%%%%%%%%%%%%%%%%%%%%%%%%%%%%%
% \usepackage{keyval}
% \usepackage[options]{hyperref}

% To add links in your PDF file, use the package "hyperref"
% with options according to your LaTeX or PDFLaTeX drivers.
%
\begin{document} 
\title{Supplementary online material:\\
The Ophiuchus DIsc Survey Employing ALMA (ODISEA). Substructures as a function of SED Class and disc mass in 100 systems}
\authorrunning{Bhowmik et al.}
\titlerunning{Substructures as a function of SED Class and disc mass in 100 systems}
\author{Trisha Bhowmik et al. \inst{\ref{instUDP},\ref{instYEMS}}}
\institute{
Instituto de Estudios Astrof\'isicos, 
Facultad de Ingenier\'ia y Ciencias,
Universidad Diego Portales,
Av. Ej\'ercito 441, Santiago, Chile
\email{trisha.bhowmik@mail.udp.cl}
\label{instUDP}
\and
Millennium Nucleus on Young Exoplanets and their Moons (YEMS), Santiago, Chile \label{instYEMS}}
\date{Received XXXX; accepted XXXX}
% }

%We use our results to provide a first-order attempt to constrain the planetary architectures that are expected to emerge from the observed disc demographics in the Ophiuchus molecular cloud.

\keywords{protoplanetary discs — circumstellar matter — stars:pre-main-sequence
— submillimetre: planetary systems — techniques: interferometric} \maketitle
%-------------------------------------------------------------------
% \onecolumn
% \twocolumn
% \include{supplementary_material/all_data_res_figures}
% \clearpage
\section*{Data and residual profiles}
% \vspace{-8mm}%

This supplementary material presents the 101 discs in our sample along with their corresponding residual images obtained after subtracting the \texttt{Frank} models from the data, using the parameters and conditions described in the main paper. The colorbars indicate the flux scale for both the data and residual images for each disc.  

As mentioned in the main text, we kept the geometrical parameters- inclination, position angle (PA), and the centering offsets ($\delta$RA and $\delta$DEC)—fixed to avoid the significant computational expense of fitting them within \texttt{Frank}. However, the residuals can be further improved when these geometrical parameters are allowed to vary. The off-centering visible in the current residual images could be reduced by exploring a grid of $\delta$RA and $\delta$DEC values, computing the residuals for each combination, and selecting the model that minimizes them. Implementing this procedure is beyond the scope of the present work due to the high computational cost. Nevertheless, we strongly encourage such refinements, particularly in small-sample analyses or detailed studies of individual discs.\\

\clearpage
% \vspace{-18mm}
\subsection*{Stage 0 and Class I/F}
\input{generated_figures_for_tex/0+I_F_data_res_figures}
\subsection*{Stage 0 and Class II}
%\clearpage
\input{generated_figures_for_tex/0+II_data_res_figures}
\clearpage
\subsection*{Stage I and Class I/F }
\input{generated_figures_for_tex/1+I_F_data_res_figures}
\subsection*{Stage I and Class II}
\input{generated_figures_for_tex/1+II_data_res_figures}
\subsection*{Stage II and Class I/F}
\input{generated_figures_for_tex/2+I_F_data_res_figures}
\subsection*{Stage II and Class II}
\input{generated_figures_for_tex/2+II_data_res_figures}
\subsection*{Stage III and Class I/F}
\input{generated_figures_for_tex/3+I_F_data_res_figures}
\subsection*{Stage III and Class II}
\input{generated_figures_for_tex/3+II_data_res_figures}
\subsection*{Stage IV and Class II}
\input{generated_figures_for_tex/4+II_data_res_figures}
\subsection*{Stage V and Class I/F}
\input{generated_figures_for_tex/5+I_F_data_res_figures}
\subsection*{Stage V and Class II }
\input{generated_figures_for_tex/5+II_data_res_figures}
\end{document}
